# Supplementary material for: Algorithm for automated tuning of a quantum dot into the single-electron regime
Source: arXiv:1911.11651 source file (2019-11-26)
Supplement: Supplementary file 1 [file SupplementaryMaterials_Algorithm_for_automated_tuning_of_a_quantum_dot_into_the_single-electron_regime.pdf]

# Supplementary material for "Algorithm for automated tuning of a quantum dot into the single-electron regime"

M. Lapointe-Major,[1] O. Germain,[2] J. Camirand Lemyre,[1] D. Lachance-Quirion,[1] S. Rochette,[1] F. Camirand Lemyre,[2] and M. Pioro-Ladrière[1]

[1)] *Institut quantique and Département de Physique, Université de Sherbrooke, Sherbrooke, Québec, J1K 2R1, Canada*

[2)] *Département de Mathématiques, Université de Sherbrooke, Sherbrooke, Québec, J1K 2R1, Canada*

## PSEUDO-CODES FOR KEY STEPS OF THE ALGORITHM

This section provides pseudo-code for the key steps performed by the algorithm.

First, algorithm 1 provides an overview of the signal processing module used to remove the background of the SET in a measured stability diagram. Next, algorithms 2 to 7 provide an overview of the image analysis module used to identify charge transition lines in a stability diagram output by the signal processing module. Finally, algorithm 8 shows the sequence of sub-diagram measurements that allows to reach the single-electron regime.

The software for algorithms 1-5,7-8 was developed using Python 2.7.10[1] and the Numpy[2], Scipy[3] and LMFIT[4] libraries. Algorithm 6 uses the C++ implementation available in Ref.[5] and is called using Python. The image analysis module is implemented in pixel coordinates with the upper-left corner of the image as the origin.

**Algorithm 1:** Signal processing module

```
Inputs:
·S {stability diagram}
for trace in S do
    fft ← Fourier transform of trace
    fft_fit ← Lorentzian fit on SET oscillations' peak
    {uses a least-square minimization algorithm}
    cutoff ← fft_fit[peak]-fft_fit[sigma]
    trace_filt ← filtered trace {applies a high-pass
    Butterworth filter of order five on trace at the
    cutoff frequency computed}
    H ← Hilbert transform of trace_filt
    H_Ω ← arctan(Im(H)/Re(H))
    {the arctan gives the angle between H and the po-
    sitive x axis in the complex plane representation}
    inst_freq ← dΩ/dV {instantaneous frequency}
    thresh ← avg(inst_freq)-3*std(inst_freq)
    {adaptative threshold to the distribution of the
    instantaneous frequency}
    trans ← where(inst_freq < thresh) {voltages
    where the instantaneous frequency is below the
    computed threshold are identified as a transition}
end for
return S_trans {S_trans is a binary image where the
value 1 is given to every pixel identified as a transi-
tion point of N and 0 otherwise}
```

**Algorithm 2:** Image analysis module

```
Inputs:
·Img {binary image of detected transition points}
Clist ← Algorithm 3 or Algorithm 6 {list of clusters}
trans_list, leftover = [], []
while Clist is not empty do
    C0 ← cluster with the smallest height over
    length ratio
    erase C0 from Clist
    temp = [C0]
    C_preselect ← list of all clusters within Clist
    within a small cone-shaped area of one of the
    endpoints of C0
    while True do
        for C in C_preselect do
            score ← algorithm 7
        end for
        if min(score) < 1 do
            C0 ← cluster associated to min(score)
            erase C0 from Clist
            temp.append(C0)
            C_preselect ← list of all clusters within
            Clist within a small cone-shaped area of
            one of the endpoints of C0
        else
            break
        end if
    end while
    if temp is a transition do
        trans_list.append(temp)
    else
        for each cluster C in temp do
            leftover.append(Cluster)
        end for
    end if
end while
return trans_list, leftover
```

**Algorithm 3:** Initial segments construction using the modified Hough transform algorithm (Algorithm from Ref.[6])

```
Inputs:
·Img {binary image of detected transition points}
Clist ← Algorithm 4 {list of clusters}
for each cluster C in Clist do
    param_C ← modified Hough transform voting
    scheme (Ref.6)
    C0, C1 ← Algorithm 5 {attempt breaking C}
    if C1 == None do
```

nothing
**else do**
errase C from Clist
Clist.*append*(C0, C1)
param_C0, param_C1 ← modified Hough transform voting scheme
**end if**
**end for**
**return** Clist

**Algorithm 4:** Linkage algorithm

**Inputs:**
·Img *{2D binary image}*,
·min_size=5 *{minimum size of each cluster of points}*,
·dist=0 *{minimum distance between clusters}*
Clist ← [] *{empty list for accepted clusters}*
leftover ← [] *{empty list for leftover points}*
**while** Img $\neq 0 \ \forall$ pixels **do**
index ← 0
group ← [] *{empty list}*
p0 ← *any*(pixel $\neq$ 0 **in** Img)
group ← *append*(p0)
Img[p0] ← 0 *{The pixel is set to 0 because it has already been accounted for}*
**while** *size*(group) > index **do**
**for** p1 = *pixel within* dist *of* group[index] **do**
**if** p1 == 1 **do**
group ← *append*(p1)
Img[p1] ← 0
**end if**
**end for**
index ← index + 1
**end while**
**if** *size*(group) < min_size **do**
leftover ← *all pixels* **in** group
**else**
Clist ← *append*(group)
**end if**
**end while**
**return** Clist, leftover

**Algorithm 5:** Dividing a cluster of points (Algorithm from Ref.[7])

**Inputs:**
·C *{cluster of points}*,
·$\vec{u}$ *{direction vector for C}*,
·$\vec{v}$ *{perpendicular vector to $\vec{u}$}*
ratio ← height over length ratio for the cluster C
*{the height is defined along $\vec{v}$ and the length along $\vec{u}$}*
$\vec{p}0$ ← *avg*(C) *{average position of all points in C}*
rot_C ← rotated cluster C
*{C is first translated by -p0 and then rotated around the origin, so that $\vec{u}' = (1,0)^T$}*
$p_-$, $p_+$ ← leftmost and rightmost points of rot_C
line($p_-$, $p_+$) ← line passing through $p_-$ and $p_+$
d ← [] *{empty list}*
**for** p **in** rot_R **do**
d ← *append*(*dist*(p, line($p_-$, $p_+$)))
**end for**
$p_{cut}$ ← *max*(d)
*C is cut in two at the pixel the farthest to line($p_-$, $p_+$)*
C0 ← all points p where $x_p < x_{p_{cut}}$
C1 ← all points p where $x_p > x_{p_{cut}}$
ratio0, ratio1 ← height over length ratios for C0 and C1
**if** (ratio0 **or** ratio1) <= ratio **do**
**return** C0, C1
**else**
**return** C, None
**end if**

**Algorithm 6:** Initial segment construction using the EDLines algorithm (Algorithm inspired from Ref.[5])

**Inputs:**
·Img *{binary image of detected transition points}*
LList <- EDLines parameter free algorithm (Ref.[5])
*{list of detected lines}*
**for** each pair (l1, l2) of lines **in** LList **do**
s ← shortest distance between the center of the
shortest cluster and the extension of the longest
d$\theta$ ← angle difference between l1 and l2
len1 ← length of the longest line
len2 ← length of the shortest line
parallel_score ← $\frac{4slen2d\theta}{\pi len1^2}$
**if** parallel_score > 1 **do**
delete shortest line
**end if**
**end for**
**for** each line l **in** LList **do**
Clist ← generate necessary cluster parameters
**end for**
**return** Clist

**Algorithm 7:** Scoring algorithm for the line reconstruction (Algorithm inspired from Ref.[7])

**Inputs:**
·C0, C1 *{clusters of points}*
·threshold = 40 *{empirical}*
s1 ← shortest distance between C0 and start point of C1
s2 ← shortest distance between C0 and center of C1
s3 ← shortest distance between C0 and end point of C1
s4 ← shortest distance between C1 and start point of C0
s5 ← shortest distance between C1 and center of C0
s6 ← shortest distance between C1 and end point of C0
s_bar ← mean(s1, s2, s3, s4, s5, s6)
**if** s_bar > threshold **do**
**return** 2 *{discard transition}*
**end if**
g ← shortest distance between endpoints of C0 and C1
d$\theta$ ← angle difference between C0 and C1
l ← length of shortest cluster
score ← $\frac{4d\theta s\_bar(g+l)}{\pi l^2}$
$\sigma_\theta \leftarrow min(\sigma_{\theta_1}, \sigma_{\theta_2})$ *{the smallest angle uncertainty of the two clusters. $\sigma_{\theta_1}$ and $\sigma_{\theta_2}$ are set to $\pi$ for EDLines}*

corr ← $d\theta/\sigma_\theta$<br>
**if** corr $> 1$ **do**<br>
    score ← score·corr<br>
    *{a penalty is added to the score if the angle difference is beyond the smallest angle uncertainty}*<br>
**end if**<br>
**return** score

**Algorithm 8:** Measurement sequence

**Inputs:**<br>
·*{requires adjusted SET gate voltages}*,<br>
·resol$_x$, resol$_y$ *{voltage resolution for the x and y axis for all stability diagram measurements}*<br>
· V_max_x, V_min_x, V_max_y, V_min_y *{voltage limits}*<br>
· V_init_x, V_init_y *{initial gate voltages}*

sp_tot = []<br>
**while** no lines found **in** last measurement **do**<br>
    trace, stab_diag ← sub-diagram measurement<br>
    sp, ia ← apply signal processing and image analysis modules<br>
    sp_tot.append(sp)<br>
    **if** line found **in** ia **do**<br>
        stab_diag ← sub-diagram measurement *{perform larger measurement centered on the detected line}*<br>
        sp, ia ← apply signal processing and image analysis modules<br>
        sp_tot.append(sp)<br>
        **if** no line found **in** ia **do**<br>
            delete previously found line *{because it was identified as an artefact}*<br>
        **end if**<br>
    **end if**<br>
**end while**<br>
**if** line found **in** ia **do**<br>
    trace, stab_diag ← sub-diagram measurement with increasing $V_{g2}$<br>
    sp, ia ← apply signal processing and image analysis modules<br>
    sp_tot.append(sp)<br>
**else if** line found **in** second last ia **do**<br>
    trace, stab_diag ← sub-diagram measurement with decreasing $V_{g1}$<br>
    sp, ia ← apply signal processing and image analysis modules<br>
    sp_tot.append(sp)<br>
**end if**<br>
transitions ← apply image analysis module on sp_tot<br>
**return** transitions[0]


[1]"Python programming language," .

[2]"Numpy - numerical computing tools for python," .

[3]"Scipy - scientific computing tools for python," .

[4]"lmfit - optimization tools for python," .

[5]C. Akinlar and C. Topal, "Edlines: A real-time line segment detector with a false detection control," Pattern Recognition Letters **32**, 1633 – 1642 (2011).

[6]L. A. Fernandes and M. M. Oliveira, "Real-time line detection through an improved hough transform voting scheme," Pattern Recognition **41**, 299 – 314 (2008).

[7]D. G. Lowe, "Three-dimensional object recognition from single two-dimensional images," Artificial Intelligence **31**, 355 – 395 (1987).
